# Supplementary material for: A Semantic Approach to Decidability in Epistemic Planning (Extended Version)
Source: arXiv:2307.15485 source file (2023-07-28)
Supplement: Supplementary file 2 [file mastar.tex]

\begin{scope}[shift={(0cm,0cm)},node distance=1.3cm, ->,>=stealth',shorten >=1pt,auto,node distance=2cm,>={Stealth[inset=0pt,length=4pt,angle'=45,round]}]

\node[event] (0) [label=below:{$e_1$}] {};

\path	
(0) edge[loop above, out=60, in=120, looseness=10] node[left] {$F = \agentSet~$}  (0)
;

\end{scope}

\begin{scope}[shift={(3cm,0cm)}, ->,>=stealth',shorten >=1pt,auto,node distance=2cm,>={Stealth[inset=0pt,length=4pt,angle'=45,round]}]

\node[event]             (0) [label=below:{$f_1$}] {}; %[label=270:$e_1$] {};
\node[event, right of=0] (1) [label=below:{$f_2$}] {};

\path	
(0) edge[<->] node[] {$P$}  (1)
(0) edge[loop left, out=150, in=210, looseness=10] node[left] {$F,P$}  (0)
(1) edge[loop right, out=-30, in=30, looseness=10] node[right] {$F,P$}  (1)
;

\end{scope}
